# Supplementary material for: Diversifying Deep Ensembles: A Saliency Map Approach for Enhanced OOD Detection, Calibration, and Accuracy
Source: arXiv:2305.11616 source file (2024-11-05)
Supplement: Supplementary file 1 [file appendix.tex]

\appendix

\begin{table*}[ht!]
\centering
\caption{OOD detection results. All methods are trained on the ID dataset and tested on multiple OOD sources. Mean and STD AUROC values are reported. The best results among different methods are \textbf{bolded}.}
\resizebox{0.75\linewidth}{!}{%
\begin{tabular}{@{}cc|cc|cccc|cc@{}}
\toprule
\multicolumn{1}{l|}{\multirow{2}{*}{\bf ID}} & \multirow{2}{*}{\bf Method} & \multicolumn{2}{c|}{\bf Near OOD} & \multicolumn{4}{c|}{\bf Far OOD} & \multicolumn{1}{l|}{\multirow{2}{*}{\bf Total Near}} & \multirow{2}{*}{\bf Total Far} \\
\multicolumn{1}{l|}{} &  & \bf Fashion MNIST & \bf NotMNIST & \bf CIFAR10 & \bf TIN & \bf Texture & \bf Places365 & \multicolumn{1}{l|}{} &  \\ \hline
\multicolumn{1}{c|}{\multirow{5}{*}{\bf \parbox[t]{2mm}{{\rotatebox[origin=c]{90}{MNIST}}}}} & DE & 95.34 \small $\pm$ 0.53 & 89.56 \small $\pm$ 0.84 & 99.06 \small $\pm$ 0.15 & 98.93 \small $\pm$ 0.18 & 96.32 \small $\pm$ 0.79 & 99.06 \small $\pm$ 0.14 & \multicolumn{1}{l|}{92.45 \small $\pm$ 0.60} & 98.34 \small $\pm$ 0.31 \\
\multicolumn{1}{l|}{} & NCL & 95.27 \small $\pm$ 0.42 & 89.19 \small $\pm$ 0.69 & 99.06 \small $\pm$ 0.11 & 98.97 \small $\pm$ 0.12 & 97.17 \small $\pm$ 0.45 & 99.03 \small \small $\pm$ 0.11 & \multicolumn{1}{l|}{92.23 \small $\pm$ 0.53} & 98.56 \small $\pm$ 0.19 \\
\multicolumn{1}{l|}{} & ADP & 96.49 \small $\pm$ 0.67 & 90.98 \small $\pm$ 0.65 & 99.48 \small $\pm$ 0.18 & 99.38 \small $\pm$ 0.21 & 97.52 \small $\pm$ 0.77 & 99.44 \small $\pm$ 0.15 & \multicolumn{1}{l|}{93.74 \small $\pm$ 0.48} & 98.96 \small $\pm$ 0.32 \\
\multicolumn{1}{l|}{} & DICE & 95.85 \small $\pm$ 0.22 & 89.88 \small $\pm$ 1.51 & 99.22 \small $\pm$ 0.19 & 99.10 \small $\pm$ 0.22 & 97.52 \small $\pm$ 1.05 & 99.20 \small $\pm$ 0.17 & \multicolumn{1}{l|}{92.87 \small $\pm$ 0.67} & 98.76 \small $\pm$ 0.41 \\
\multicolumn{1}{l|}{} & \textbf{SDDE (Our)} & \bf 98.85 \small $\pm$ 0.38 & \bf 94.27 \small $\pm$ 1.32 & \bf 99.88 \small $\pm$ 0.03 & \bf 99.84 \small $\pm$ 0.03 & \bf 99.97 \small $\pm$ 0.01 & \bf 99.82 \small $\pm$ 0.04 & \multicolumn{1}{l|}{\bf 96.56 \small $\pm$ 0.67} & \bf 99.88 \small $\pm$ 0.02 \\ \hline
\multicolumn{2}{c|}{} & \bf CIFAR100 & \bf TIN & \bf MNIST & \bf SVHN & \bf Texture & \bf Places365 & \multicolumn{2}{l}{} \\ \hline
\multicolumn{1}{c|}{\multirow{5}{*}{\bf \parbox[t]{2mm}{{\rotatebox[origin=c]{90}{CIFAR10}}}}} & DE & 90.31 \small $\pm$ 0.23 & 91.84 \small $\pm$ 0.16 & 95.35 \small $\pm$ 0.53 & 95.05 \small $\pm$ 0.47 & 92.52 \small $\pm$ 0.30 & 91.29 \small $\pm$ 0.59 & \multicolumn{1}{l|}{91.07 \small $\pm$ 0.17} & 93.55 \small $\pm$ 0.20 \\
\multicolumn{1}{l|}{} & NCL & 90.51 \small $\pm$ 0.12 & 91.93 \small $\pm$ 0.08 & 95.09 \small $\pm$ 0.29 & 94.81 \small $\pm$ 0.46 & 92.18 \small $\pm$ 0.34 & 92.00 \small $\pm$ 0.26 & \multicolumn{1}{l|}{91.22 \small $\pm$ 0.09} & 93.52 \small $\pm$ 0.17 \\
\multicolumn{1}{l|}{} & ADP & 89.96 \small $\pm$ 0.25 & 91.62 \small $\pm$ 0.13 & 95.41 \small $\pm$ 0.24 & 94.66 \small $\pm$ 0.40 & 92.55 \small $\pm$ 0.12 & 91.38 \small $\pm$ 0.53 & \multicolumn{1}{l|}{90.79 \small $\pm$ 0.17} & 93.50 \small $\pm$ 0.16 \\
\multicolumn{1}{l|}{} & DICE & 89.09 \small $\pm$ 0.79 & 90.89 \small $\pm$ 0.48 & 94.46 \small $\pm$ 1.10 & 94.89 \small $\pm$ 0.49 & 92.36 \small $\pm$ 0.45 & 89.84 \small $\pm$ 1.14 & \multicolumn{1}{l|}{89.99 \small $\pm$ 0.63} & 92.89 \small $\pm$ 0.47 \\
\multicolumn{1}{l|}{} & \textbf{SDDE (Our)} & \bf 91.20 \small $\pm$ 0.13 & \bf 92.92 \small $\pm$ 0.17 & \bf 96.77 \small $\pm$ 0.45 & \bf 95.74 \small $\pm$ 0.36 & \bf 92.69 \small $\pm$ 0.62 & \bf 93.19 \small $\pm$ 0.62 & \multicolumn{1}{l|}{\bf 92.06 \small $\pm$ 0.13} & \bf 94.60 \small $\pm$ 0.17 \\
\hline
\multicolumn{2}{c|}{} & \bf CIFAR10 & \bf TIN & \bf MNIST & \bf SVHN & \bf Texture & \bf Places365 & \multicolumn{2}{l}{} \\ \hline
\multicolumn{1}{c|}{\multirow{5}{*}{\bf \parbox[t]{2mm}{{\rotatebox[origin=c]{90}{CIFAR100}}}}} & DE & 80.83 \small $\pm$ 0.55 & 84.28 \small $\pm$ 0.52 & 80.24 \small $\pm$ 1.43 & 81.09 \small $\pm$ 1.27 & 80.16 \small $\pm$ 0.41 & 80.96 \small $\pm$ 0.26 & \multicolumn{1}{l|}{82.55 \small $\pm$ 0.51} & 80.61 \small $\pm$ 0.51 \\
\multicolumn{1}{l|}{} & NCL & 81.11 \small $\pm$ 0.20 & 84.48 \small $\pm$ 0.19 & 79.66 \small $\pm$ 0.66 & 80.91 \small $\pm$ 1.99 & 80.30 \small $\pm$ 0.52 & 81.24 \small $\pm$ 0.17 & \multicolumn{1}{l|}{82.79 \small $\pm$ 0.18} & 80.53 \small $\pm$ 0.66 \\
\multicolumn{1}{l|}{} & ADP & 81.12 \small $\pm$ 0.19 & 84.85 \small $\pm$ 0.22 & 79.54 \small $\pm$ 0.76 & 82.84 \small $\pm$ 2.16 & 81.80 \small $\pm$ 0.47 & 81.28 \small $\pm$ 0.11 & \multicolumn{1}{l|}{82.98 \small $\pm$ 0.18} & 81.37 \small $\pm$ 0.54 \\
\multicolumn{1}{l|}{} & DICE & 81.42 \small $\pm$ 0.18 & 84.94 \small $\pm$ 0.21 & \bf 83.37 \small $\pm$ 1.11 & 82.40 \small $\pm$ 1.96 & 81.43 \small $\pm$ 0.39 & 81.41 \small $\pm$ 0.27 & \multicolumn{1}{l|}{83.18 \small $\pm$ 0.14} & 82.15 \small $\pm$ 0.85 \\
\multicolumn{1}{l|}{} & \textbf{SDDE (Our)} & \bf 81.97 \small $\pm$ 0.10 & \bf 85.34 \small $\pm$ 0.16 & 81.86 \small $\pm$ 1.80 & \bf 83.40 \small $\pm$ 1.03 & \bf 82.67 \small $\pm$ 0.35 & \bf 81.63 \small $\pm$ 0.18 & \multicolumn{1}{l|}{\bf 83.65 \small $\pm$ 0.09} & \bf 82.39 \small $\pm$ 0.56 \\
\bottomrule
\end{tabular}
}
\label{tab:ood-full}
\end{table*}

\begin{table*}[h!]
\caption{Diversity loss ablation study.}
\label{tab:adversarial}
\begin{center}
\resizebox{0.75\textwidth}{!}{
\begin{tabular}{l|l|cccccc}
\hline
\textbf{Dataset} & \textbf{Method}     & \textbf{Near ODD $\uparrow$} & \textbf{Far OOD $\uparrow$} & \textbf{NLL ($\times 10$) $\downarrow$} & \textbf{ECE ($\times 10^2$) $\downarrow$} & \textbf{Brier score ($\times 10^2$) $\downarrow$} & \textbf{Accuracy (\%) $\uparrow$}   \\
\hline
\multirow{2}{*}{MNIST} & 
DE  & 92.45 \small $\pm$ 0.60 & 98.34 \small $\pm$ 0.31 & 0.38 \small $\pm$ 0.02 & \bf 0.21 \small $\pm$ 0.06 & 1.95 \small $\pm$ 0.09 & 98.72 \small $\pm$ 0.07 \\ 
& DE with $\mathcal{L}_{adv}$   & \bf 95.63 \small $\pm$ 0.46 & \bf 99.55 \small $\pm$ 0.02 & \bf 0.34 \small $\pm$ 0.01 & 0.26 \small $\pm$ 0.04 & \bf 1.76 \small $\pm$ 0.05 & \bf 98.84 \small $\pm$ 0.06 \\
\hline
\multirow{2}{*}{CIFAR10} & 
DE  & \bf 91.07 \small $\pm$ 0.17 & \bf 93.55 \small $\pm$ 0.20 & \bf 1.30 \small $\pm$ 0.02 & \bf 0.84 \small $\pm$ 0.16 & \bf 5.96 \small $\pm$ 0.08 & \bf 96.07 \small $\pm$ 0.10\\ 
& DE with $\mathcal{L}_{adv}$   & 90.84 \small $\pm$ 0.13 & 92.12 \small $\pm$ 0.22 & 2.02 \small $\pm$ 0.04 & 0.93 \small $\pm$ 0.09 & 9.60 \small $\pm$ 0.15 & 93.50 \small $\pm$ 0.21 \\
\hline
\multirow{2}{*}{CIFAR100} & 
DE  & \bf 82.55 \small $\pm$ 0.51 & \bf 80.61 \small $\pm$ 0.51 & \bf 7.21 \small $\pm$ 0.14 & 3.78 \small $\pm$ 0.17 & \bf 27.33 \small $\pm$ 0.76 & \bf 80.95 \small $\pm$ 0.54 \\ 
& DE with $\mathcal{L}_{adv}$   & 80.87 \small $\pm$ 0.60 & 76.87 \small $\pm$ 0.99 & 10.06 \small $\pm$ 0.05 & \bf 3.11 \small $\pm$ 0.79 & 37.00 \small $\pm$ 0.35 & 72.74 \small $\pm$ 0.39 \\
\hline
\end{tabular}
}
\end{center}
\end{table*}

\begin{table*}[h]
\caption{Comparison of saliency map computation algorithms.}
\label{tab:maps}
\begin{center}
\resizebox{0.75\textwidth}{!}{
\begin{tabular}{l|l|cccccc}
\hline
\textbf{Dataset} & \textbf{Method}     & \textbf{Near ODD $\uparrow$} & \textbf{Far OOD $\uparrow$} & \textbf{NLL ($\times 10$) $\downarrow$} & \textbf{ECE ($\times 10^2$) $\downarrow$} & \textbf{Brier score ($\times 10^2$) $\downarrow$} & \textbf{Accuracy (\%) $\uparrow$}   \\
\hline
\multirow{2}{*}{MNIST} & 
Inp. grad.  & 92.04 \small $\pm$ 0.57 & 98.59 \small $\pm$ 0.30 & \bf 0.37 \small $\pm$ 0.02 & \bf 0.28 \small $\pm$ 0.40 & \bf 1.92 \small $\pm$ 0.09 & \bf 98.79 \small $\pm$ 0.05 \\ 
& GradCAM & \bf 96.56 \small $\pm$ 0.67 & \bf 99.88 \small $\pm$ 0.02 & \bf 0.37 \small $\pm$ 0.03 & \bf 0.28 \small $\pm$ 0.08 & \bf 1.92 \small $\pm$ 0.15 & 98.73 \small $\pm$ 0.14 \\
\hline
\multirow{2}{*}{CIFAR10} & 
Inp. grad.  & 91.18 \small $\pm$ 0.13 & 93.56 \small $\pm$ 0.24 & 1.35 \small $\pm$ 0.05 & \bf 0.76 \small $\pm$ 0.12 & 6.23 \small $\pm$ 0.34 & 95.89 \small $\pm$ 0.21 \\ 
& GradCAM & \bf 92.06 \small $\pm$ 0.13 & \bf 94.60 \small $\pm$ 0.17 & \bf 1.28 \small $\pm$ 0.01 & 0.82 \small $\pm$ 0.15 & \bf 5.88 \small $\pm$ 0.07 & \bf 96.08 \small $\pm$ 0.11 \\
\hline
\multirow{2}{*}{CIFAR100} & 
Inp. grad. & 82.80 \small $\pm$ 0.18 & 80.06 \small $\pm$ 0.58 & 7.14 \small $\pm$ 0.03 & 3.76 \small $\pm$ 0.26 & 27.06 \small $\pm$ 0.27 & 81.06 \small $\pm$ 0.14 \\ 
& GradCAM & \bf 83.69 \small $\pm$ 0.08 & \bf 82.39 \small $\pm$ 0.50 & \bf 6.93 \small $\pm$ 0.05 & \bf 3.45 \small $\pm$ 0.35 & \bf 26.66 \small $\pm$ 0.33 & \bf 81.27 \small $\pm$ 0.24 \\
\hline
\end{tabular}
}
\end{center}
\end{table*}

\section{Detailed OOD Detection Table}

The OOD detection performance for each dataset in Near And far OOD detection AUROC of SDDE and the baselines are reported in Table \ref{tab:ood-full}. It can be seen that SDDE provides a consistent performance boost in 17 of 18 comparisons.

\section{Additional Diversity Metrics}\label{app:fulldiversity}

\begin{table*}[h]
\centering
\caption{Diversification metrics. The best result in each column is \textbf{bolded}. The DICE method failed to converge on ImageNet.}
\resizebox{0.75\linewidth}{!}{%
\begin{tabular}{@{}cc|ccccc|cc@{}}
\toprule
\multirow{2}{*}{\bf Dataset} & \multirow{2}{*}{\bf Method} & \multicolumn{5}{c|}{\bf Diversity} & \multicolumn{2}{c}{\bf Error} \\
& & \bf Disagreement$\uparrow$ & \bf Correlation$\downarrow$ & \bf Q-value$\downarrow$ & \bf D/S Error Rate$\uparrow$ & \bf MI$\downarrow$ & \bf Mean & \bf Ensemble \\
\hline
\multirow{5}{*}{\bf \parbox[t]{2mm}{{\rotatebox[origin=c]{90}{CIFAR 10}}}} 
 & DE & 4.37 \small $\pm$ 0.26 & 58.85 \small $\pm$ 1.43 & 97.38 \small $\pm$ 0.31 & 0.22 \small $\pm$ 0.02 & 2.06 \small $\pm$ 0.01 & 4.89 \small $\pm$ 0.13 & 3.93 \small $\pm$ 0.10 \\
 & NCL & 4.32 \small $\pm$ 0.16 & 59.92 \small $\pm$ 0.81 & 97.53 \small $\pm$ 0.17 & 0.22 \small $\pm$ 0.01 & 2.07 \small $\pm$ 0.01 & 4.95 \small $\pm$ 0.13 & 4.04 \small $\pm$ 0.08 \\
 & ADP & \bf 4.89 \small $\pm$ 0.06 & \bf 57.52 \small $\pm$ 0.39 & \bf 97.03 \small $\pm$ 0.09 & \bf 0.32 \small $\pm$ 0.01 & \bf 2.04 \small $\pm$ 0.00 & 5.14 \small $\pm$ 0.04 & 3.93 \small $\pm$ 0.12 \\
 & DICE & 4.88 \small $\pm$ 1.01 & 57.61 \small $\pm$ 4.15 & 96.82 \small $\pm$ 1.32 & 0.25 \small $\pm$ 0.05 & \bf 2.04 \small $\pm$ 0.04 & 5.24 \small $\pm$ 0.57 & 4.10 \small $\pm$ 0.16 \\
 & SDDE & 4.33 \small $\pm$ 0.13 & 59.29 \small $\pm$ 0.95 & 97.47 \small $\pm$ 0.18 & 0.23 \small $\pm$ 0.01 & 2.07 \small $\pm$ 0.01 & \bf 4.87 \small $\pm$ 0.11 & \bf 3.92 \small $\pm$ 0.11 \\
\hline
\multirow{5}{*}{\bf \parbox[t]{2mm}{{\rotatebox[origin=c]{90}{CIFAR 100}}}}
 & DE & 20.81 \small $\pm$ 2.09 & 62.90 \small $\pm$ 2.25 & 92.70 \small $\pm$ 1.42 & 0.86 \small $\pm$ 0.10 & 3.63 \small $\pm$ 0.09 & 23.12 \small $\pm$ 1.28 & 19.05 \small $\pm$ 0.54 \\
 & NCL & 20.57 \small $\pm$ 0.93 & 63.06 \small $\pm$ 1.32 & 92.86 \small $\pm$ 0.70 & 0.83 \small $\pm$ 0.04 & 3.64 \small $\pm$ 0.04 & 23.00 \small $\pm$ 0.47 & 19.08 \small $\pm$ 0.20 \\
 & ADP & \bf 25.53 \small $\pm$ 0.28 & 63.02 \small $\pm$ 0.78 & 92.44 \small $\pm$ 0.40 & \bf 1.78 \small $\pm$ 0.08 & \bf 3.43 \small $\pm$ 0.01 & 25.13 \small $\pm$ 0.12 & 18.82 \small $\pm$ 0.06 \\
 & DICE & 21.98 \small $\pm$ 0.31 & \bf 60.88 \small $\pm$ 0.41 & \bf 91.78 \small $\pm$ 0.26 & 0.98 \small $\pm$ 0.01 & 3.59 \small $\pm$ 0.01 & 23.20 \small $\pm$ 0.25 & 18.74 \small $\pm$ 0.25 \\
 & SDDE & 21.00 \small $\pm$ 1.34 & 61.43 \small $\pm$ 1.94 & 92.09 \small $\pm$ 1.13 & 0.86 \small $\pm$ 0.07 & 3.63 \small $\pm$ 0.05 & \bf 22.80 \small $\pm$ 0.63 & \bf 18.67 \small $\pm$ 0.25 \\
 \hline
 \multirow{5}{*}{\bf \parbox[t]{2mm}{{\rotatebox[origin=c]{90}{\hspace{0.13in}ImageNet}}}}
 & DE & 4.37 \small $\pm$ 0.02 & 93.65 \small $\pm$ 0.03 & 99.84 \small $\pm$ 0.00 & 0.09 \small $\pm$ 0.00 & 5.99 \small $\pm$ 0.00 & 25.41 \small $\pm$ 0.00 & 24.84 \small $\pm$ 0.06\\
 & NCL & 0.51 \small $\pm$ 0.02 & 99.31 \small $\pm$ 0.03 & 100.00 \small $\pm$ 0.00 & 0.01 \small $\pm$ 0.00 & 6.17 \small $\pm$ 0.00 & 25.41 \small $\pm$ 0.11 & 24.95 \small $\pm$ 0.13\\
 & ADP & \bf 30.17 \small $\pm$ 0.47 & \bf 80.93 \small $\pm$ 0.67 & \bf 98.05 \small $\pm$ 0.10 & \bf 2.43 \small $\pm$ 0.04 & \bf 4.50 \small $\pm$ 0.03 & 34.56 \small $\pm$ 0.20 &  24.90 \small $\pm$ 0.01 \\
 & SDDE& 4.36 \small $\pm$ 0.07 & 93.80 \small $\pm$ 0.09 & 99.85 \small $\pm$ 0.00 & 0.09 \small $\pm$ 0.00 & 5.99 \small $\pm$ 0.00 & \bf 25.39 \small $\pm$ 0.00 & \bf 24.80 \small $\pm$ 0.01\\
\bottomrule
\end{tabular}%
}
\label{tab:diversity-full}
\end{table*}

\section{Adversarial Loss in Deep Ensembles}
\label{ap:advloss}
The original Deep Ensemble approach \cite{lakshminarayanan2017deepensemble} applied an extra adversarial loss, which is not present in OpenOOD. Therefore, we evaluate the impact of this loss on accuracy, calibration and OOD detection scores. The adversarial loss is inspired by adversarial samples generation and has the following form:
\begin{equation}
    \mathcal{L}_{adv} = \frac{1}{N}\sum\limits_k\mathcal{L}_{CE}(\hat{x}_k, y, \theta_k),
\end{equation}
where $\hat{x}_k$ is an adversarial version of the input image $x$ with label $y$, computed as
\begin{equation}
    \hat{x}_k = x + \epsilon \sign\left(\nabla_{x}\mathcal{L}_{CE}(x, y, \theta_k)\right).
\end{equation}
We follow the original implementation and set $\epsilon$ equal to $0.01$ of the input data's dynamic range.

We evaluated the adversarial loss for the CIFAR-10 and CIFAR-100 datasets. According to our results, presented in Table \ref{tab:adversarial}, adversarial loss slightly reduces the quality of the ensemble. We conclude that adversarial loss improves ensemble robustness to adversarial samples, but negatively affects accuracy and OOD detection.

\section{Input Gradients vs GradCAM}
\label{ap:inpgrad}
In this work, we diversify saliency maps computed by GradCAM. We also evaluate saliency maps constructed by taking gradients w.r.t. the input image, i.e. {\it input gradients} \cite{simonyan2013saliencegrad}. The results from \mbox{Table \ref{tab:maps}} demonstrate the superiority of GradCAM to input gradients in terms of OOD detection and classification accuracy. 

Another difference between input gradients and GradCAM lies in computation speed. Diversity loss requires two backward passes: one for making a saliency map, and another for loss optimization. The complexity of both passes depends on the method used. Computing gradients w.r.t. the input images requires a backward pass through all layers, while GradCAM stops when the feature extraction layer is reached. This leads to a difference in training speed, making GradCAM about 2.4 times faster than input gradients. As GradCAM outperforms input gradients in both accuracy and training speed, we decided to use it as a default choice for ensemble diversification.

\section{Wide ResNet-28-10 Experiments}
\label{ap:wrn}

In addition to OpenOOD benchmarks, we conducted experiments with the Wide ResNet architecture. The results in Table \ref{tab:wrn-18} show that SDDE with WRN-28-10 outperforms other methods in terms of accuracy, calibration, and OOD detection scores.

\begin{table*}[h!]
\centering
\caption{Wide ResNet 28-10 results.}
\resizebox{.75\textwidth}{!}{%
\begin{tabular}{cc|cccccc}
\toprule
\bf Dataset & \bf Method & Near OOD & Far OOD & NLL & ECE & Brier & Accuracy \\
\hline
\multirow{5}{*}{\bf \parbox[t]{2mm}{{\rotatebox[origin=c]{90}{CIFAR 10}}}}
& DE & 90.31 \small $\pm$ 0.18 & 93.70 \small $\pm$ 0.18 & 11.87 \small $\pm$ 0.10 & \bf 0.94 \small $\pm$ 0.14 & 5.27 \small $\pm$ 0.11 & 96.59 \small $\pm$ 0.15 \\
& NCL & 90.26 \small $\pm$ 0.37 & 93.44 \small $\pm$ 0.20 & 12.20 \small $\pm$ 0.34 & 0.78 \small $\pm$ 0.16 & 5.39 \small $\pm$ 0.24 & 96.48 \small $\pm$ 0.19 \\
& ADP & 88.81 \small $\pm$ 0.49 & 92.86 \small $\pm$ 0.41 & 12.77 \small $\pm$ 0.29 & 0.75 \small $\pm$ 0.12 & 5.39 \small $\pm$ 0.15 & 96.57 \small $\pm$ 0.12 \\
& DICE & 87.37 \small $\pm$ 0.39 & 91.52 \small $\pm$ 0.20 & 14.44 \small $\pm$ 0.32 & 1.09 \small $\pm$ 0.10 & 6.03 \small $\pm$ 0.18 & 96.17 \small $\pm$ 0.16 \\
& SDDE (Our) & \bf 90.40 \small $\pm$ 0.23 & \bf 94.30 \small $\pm$ 0.22 & \bf 11.80 \small $\pm$ 0.17 & \bf 0.94 \small $\pm$ 0.15 & \bf 5.16 \small $\pm$ 0.11 & \bf 96.65 \small $\pm$ 0.06 \\
\hline
\multirow{5}{*}{\bf \parbox[t]{2mm}{{\rotatebox[origin=c]{90}{CIFAR 100}}}}
& DE & 83.03 \small $\pm$ 0.20 & 81.27 \small $\pm$ 0.69 & 66.32 \small $\pm$ 0.47 & 3.55 \small $\pm$ 0.30 & 24.48 \small $\pm$ 0.35 & 82.99 \small $\pm$ 0.33 \\
& NCL & 83.02 \small $\pm$ 0.23 & 80.47 \small $\pm$ 0.20 & 66.46 \small $\pm$ 0.54 & 3.49 \small $\pm$ 0.30 & 24.45 \small $\pm$ 0.09 & 83.05 \small $\pm$ 0.11 \\
& ADP & 82.48 \small $\pm$ 0.26 & 79.78 \small $\pm$ 0.98 & 70.75 \small $\pm$ 0.55 & 3.50 \small $\pm$ 0.11 & 24.85 \small $\pm$ 0.33 & 83.02 \small $\pm$ 0.22 \\
& DICE & 82.17 \small $\pm$ 0.78 & 80.11 \small $\pm$ 1.17 & 72.36 \small $\pm$ 0.97 & 3.99 \small $\pm$ 0.12 & 25.46 \small $\pm$ 0.57 & 82.56 \small $\pm$ 0.56 \\
& SDDE (Our) & \bf 83.54 \small $\pm$ 0.12 & \bf 82.81 \small $\pm$ 0.42 & \bf 65.66 \small $\pm$ 0.20 & \bf 3.39 \small $\pm$ 0.09 & \bf 24.17 \small $\pm$ 0.14 & \bf 83.34 \small $\pm$ 0.15 \\
\bottomrule
\end{tabular}%
}
\label{tab:wrn-18}
\end{table*}

\section{Number of Models}
\label{ap:nummodels}
The key parameter of any ensemble is its number of models. A large ensemble usually provides a better confidence estimate, but its size negatively affects the computation speed. In order to determine the best number of models to use without incurring losses, we analyze the dependency of quality on ensemble size. The results for classification and OOD detection quality are presented in Figure \ref{fig:nmodels}. It can be seen that SDDE effectively uses multiple models, leading to better results for all ensemble sizes, starting from 3 in the CIFAR-10 and CIFAR-100 Near and Far setups.

\begin{figure}[ht!]
\centerline{\includegraphics[width=1.1\linewidth]{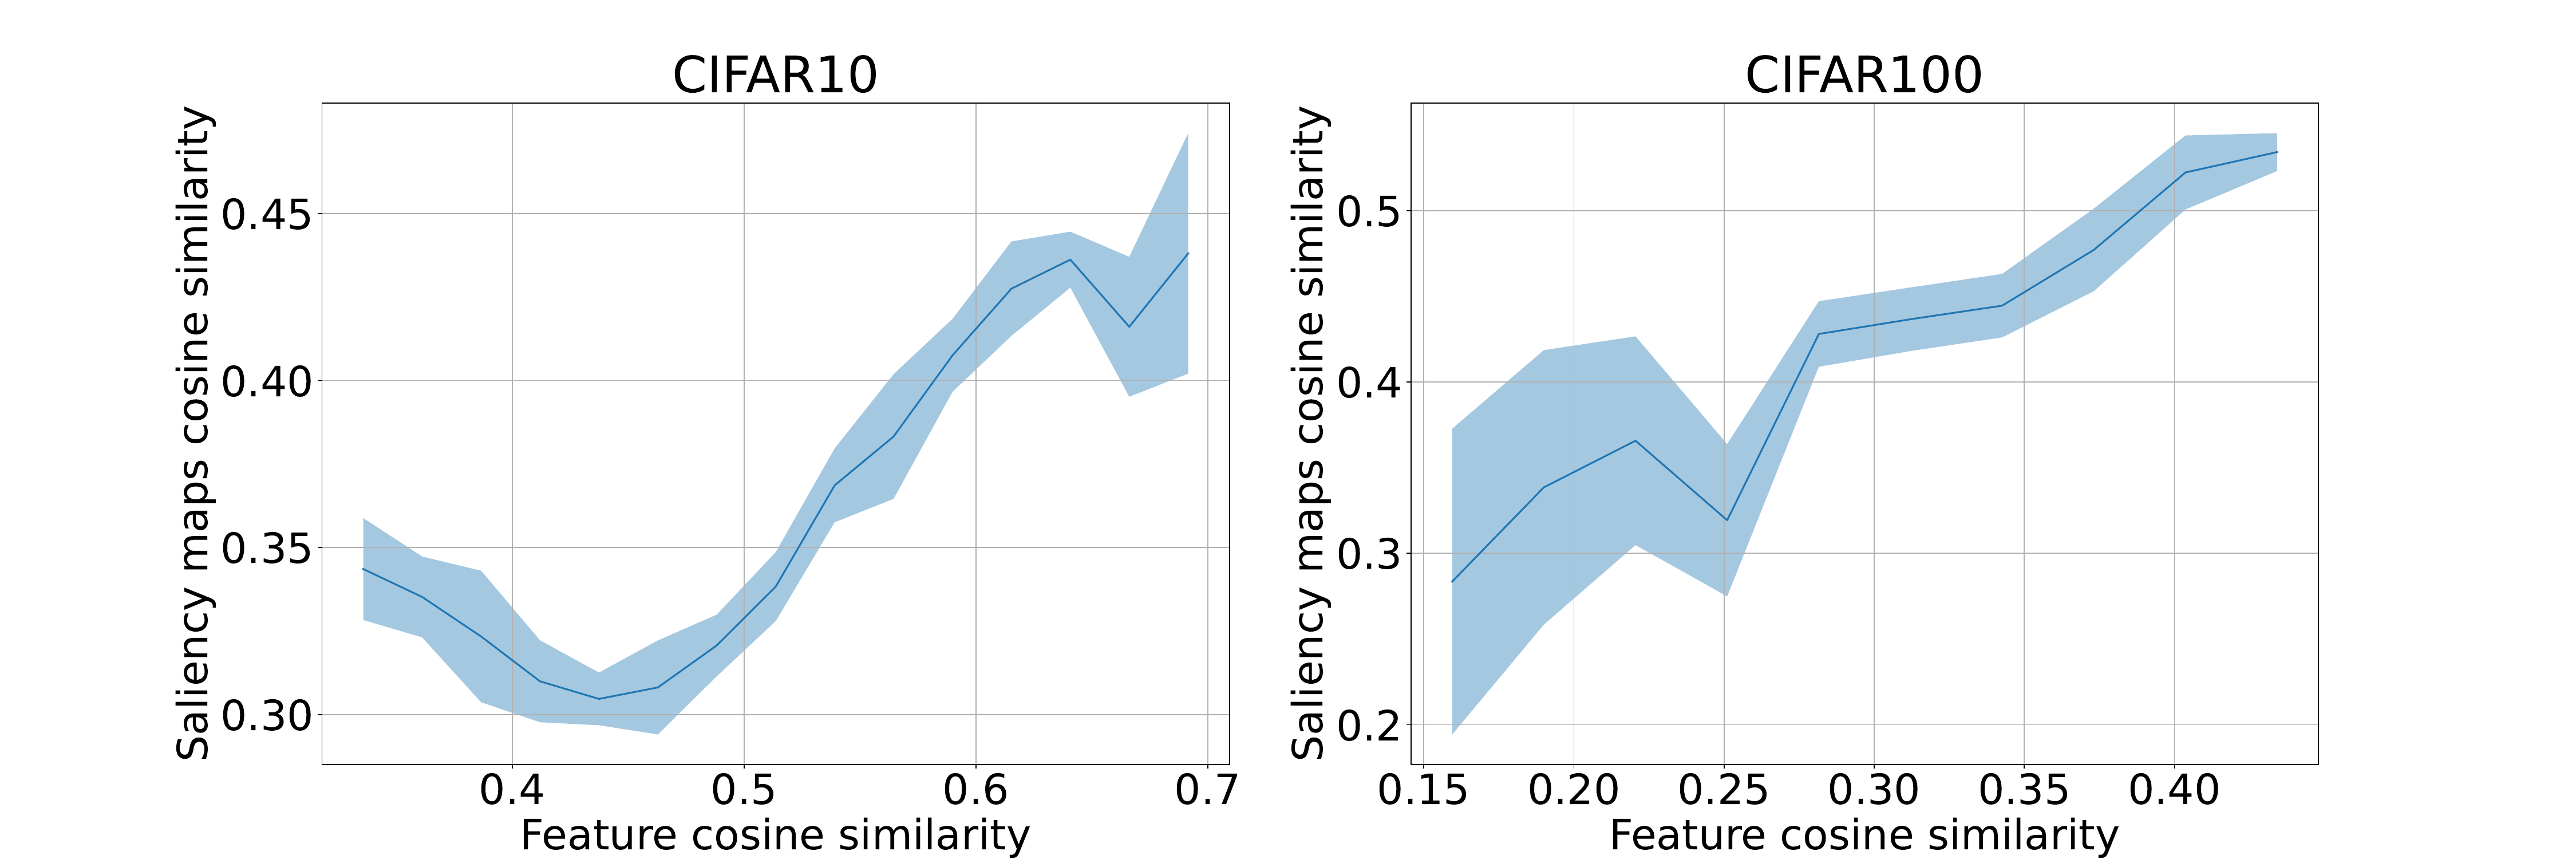}}
\caption{The dependency of ensemble saliency maps cosine similarity on feature cosine similarities. Saliency maps are computed using GradCAM. Mean and STD values w.r.t. multiple training seeds for the CIFAR10/100 datasets are reported.}
\label{fig:feat-vs-map}
\end{figure}

\begin{figure*}[h]
\centerline{\includegraphics[width=\linewidth]{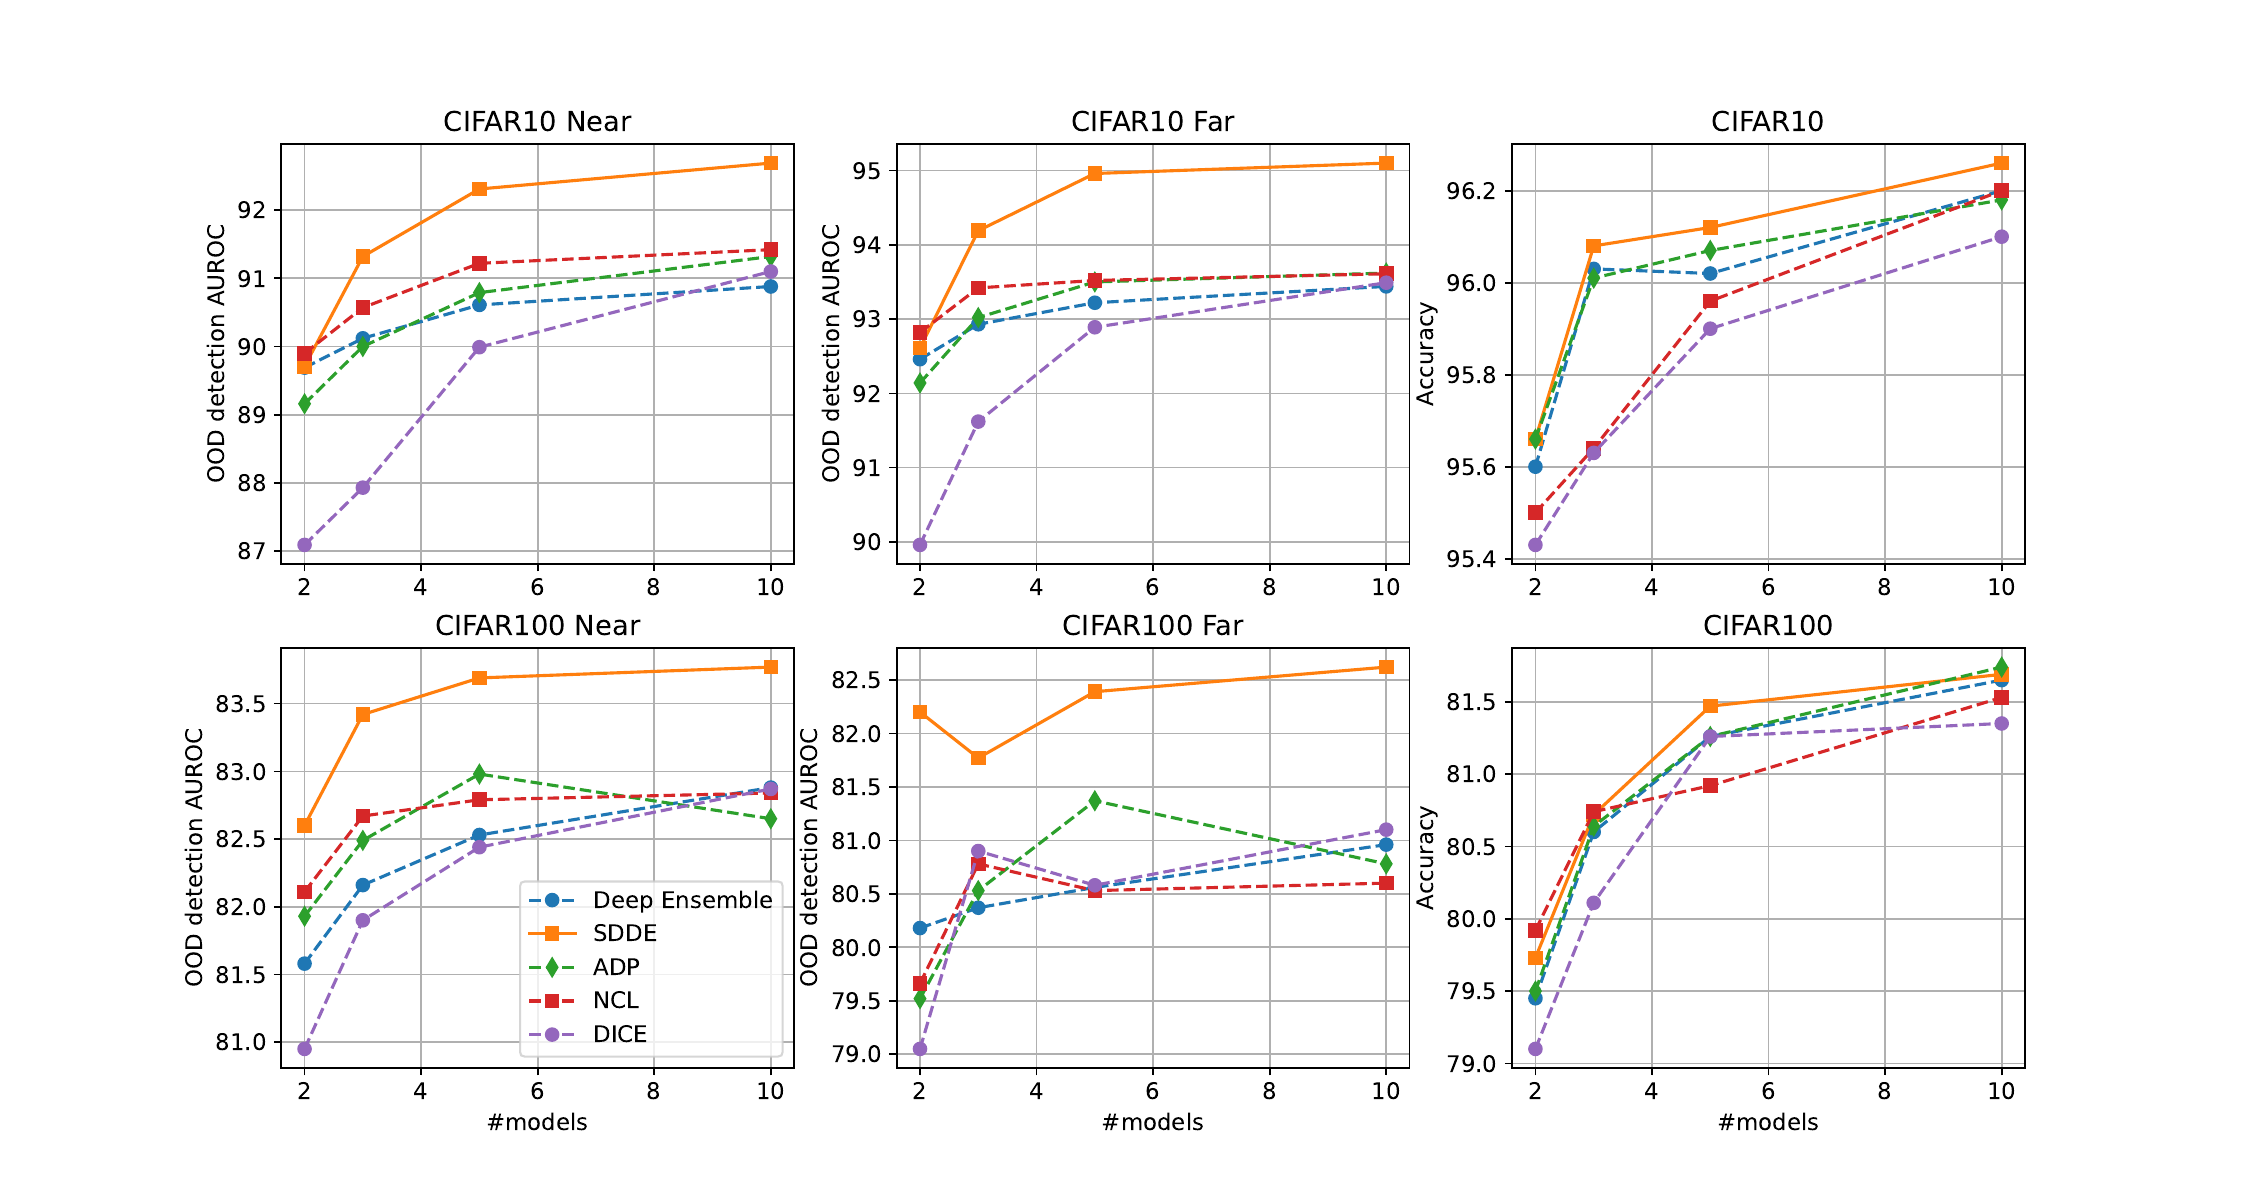}}
\caption{Classification accuracy and OOD detection quality depending on ensemble size.}
\label{fig:nmodels}
\end{figure*}

\section{Saliency Maps vs Feature Diversity}\label{app:diversity}

In Section \ref{sec:toy}, we established a link between the diversity observed in saliency maps space and the diversity in the prediction space of models. However, an unresolved question remains: does the diversity in saliency maps contribute to diversity in the feature space? To address this, we analyzed the cosine similarities between the saliency maps and the models' penultimate layers' features. The findings are depicted in Figure \ref{fig:feat-vs-map}. It's evident from the data that higher similarities in the feature space correspond to increased similarities in saliency maps. Consequently, we infer that enhancing the diversity of saliency maps compels ensemble models to utilize distinct features for making predictions.

\section{Logit Aggregation Ablation for SDDE\textsubscript{OOD}}

Following Section \ref{sec:logits_sdde_odd}, we ablate logit aggregation strategy for SDDE\textsubscript{OOD} method. The results are presented in Table \ref{tab:malablood}. It can be seen that SDDE\textsubscript{OOD} outperforms the baselines with MAL aggregation in 4 out 6 cases.

\begin{table*}[h!]
\caption{Comparison of OOD score aggregation methods for the SDDE\textsubscript{OOD} method.}
\centering
\label{tab:malablood}
\resizebox{0.75\textwidth}{!}{
\begin{tabular}{@{}cl|ll|ll|ll@{}}
\toprule
\multicolumn{2}{c|}{\multirow{2}{*}{Method}} & \multicolumn{2}{c|}{CIFAR10} & \multicolumn{2}{c|}{CIFAR100} & \multicolumn{2}{c}{ImageNet200} \\ \cmidrule(l){3-8} 
\multicolumn{2}{c|}{} & \multicolumn{1}{c}{Near} & \multicolumn{1}{c|}{Far} & \multicolumn{1}{c}{Near} & \multicolumn{1}{c|}{Far} & \multicolumn{1}{c}{Near} & \multicolumn{1}{c}{Far} \\ \midrule
\multicolumn{2}{l|}{OE-Ensemble\textsubscript{MSP}} & 96.25 ± 0.14 & 97.34 ± 0.14 & 89.40 ± 0.02 & \textbf{88.34 ± 0.72} & 84.05 ± 0.19 & 88.77 ± 0.37 \\
\multicolumn{2}{l|}{OE-Ensemble\textsubscript{MAL}} & \bf 96.27 ± 0.01 & 97.40 ± 0.19 & 89.59 ± 0.04 & 84.41 ± 0.97 & 84.41 ± 0.15 & 89.45 ± 0.26 \\
\multicolumn{2}{c|}{\textbf{SDDE\textsubscript{MSP}}} & \textbf{96.27 ± 0.07} & 95.57 ± 0.05 & 89.64 ± 0.17 & 85.38 ± 1.76 & 84.10 ± 0.10 & 88.95 ± 0.15 \\
\multicolumn{2}{c|}{\textbf{SDDE\textsubscript{MAL}}} & 96.22 ± 0.08 & \textbf{97.60 ± 0.08} & \textbf{89.70 ± 0.22} & 85.47 ± 1.76 & \textbf{84.46 ± 0.07} & \textbf{89.57 ± 0.11} \\ \bottomrule
\end{tabular}}
\end{table*}

\section{Computational Complexity}

We have conducted a comparative analysis of the computational cost of SDDE training compared to other methods. According to our measurements on the NVIDIA V100 GPU, with training details described in Section \ref{sec:details} on CIFAR10, training a single SDDE model takes 2.9 hours using a single V100 GPU. Deep Ensemble takes 6.4 hours, and Deep Ensemble without adversarial loss takes 1.4 hours. The inference time is not affected by diversity loss and remains identical for all ensemble methods. Similarly, during training, SDDE, Deep Ensemble, and Deep Ensemble without adversarial loss consume 6.2 GB, 6.8 GB, and 3.9 GB of GPU memory, respectively.

\section{SDDE Training Algorithm}\label{app:listing}

SDDE training algorithm is presented in Listing \ref{lst:ded}. During cross-entropy (CE) loss computation, each model receives its own batch. The diversity loss is computed for a single batch, forwarded through each model. The training procedure with OOD sample is presented in Listing \ref{lst:babka}. The loss is extended with Outlier Exposure (OE) objective \cite{hendrycks2018oe}, computed on the OOD batch.
Similar to OE training, both in-distribution and OOD batches are concatenated and processed via single forward pass. This way, batch normalization statistics are adapted to OOD data.
\begin{algorithm}[h!]
\caption{SDDE training}\label{lst:ded}
\begin{algorithmic}[1]
\Require{$\mathcal{D}$, $N$, $T$, $\lambda$, $\epsilon$}
\Ensure{Trained weights $\theta_k, k \in \overline{1, N}$}
\Statex
\State Initialize $\theta_k, k \in \overline{1, N}$
\For{$i \gets 1$ to $T$}
    \State $l \gets 0$
    \For{$k \gets 1$ to $N$}
        \State Sample batch $(x^i_k, y^i_k)$ from $\mathcal{D}$
        \State $l \gets l + \frac{1}{N} \mathcal{L}_{CE}(x^i_k, y^i_k; \theta_k)$
    \EndFor
    \State Sample batch $(\hat x_k, \hat y_k)$ from $\mathcal{D}$
    \State $l \gets l + \lambda \mathcal{L}_{div}(\hat x_k, \hat y_k; \theta_1, \dots, \theta_N)$
    \For{$k \gets 1$ to $N$}
        \State $\theta_k \gets \theta_k - \epsilon \nabla_{\theta_k}l$
    \EndFor
\EndFor
\end{algorithmic}
\end{algorithm}
%\end{minipage}\hfill
%\begin{minipage}[t]{.56\textwidth}
\begin{algorithm}[h!]
\caption{SDDE training with OOD data}\label{lst:babka}
\begin{algorithmic}[1]
\Require{$\mathcal{D}$, $\mathcal{D}_{OOD}$, $N$, $T$, $\lambda$, $\epsilon$}
\Ensure{Trained weights $\theta_k, k \in \overline{1, N}$}
\Statex
\State Initialize $\theta_k, k \in \overline{1, N}$
\For{$i \gets 1$ to $T$}
    \State $l \gets 0$
    \For{$k \gets 1$ to $N$}
        \State Sample batch $(x^i_k, y^i_k)$ from $\mathcal{D}$
        \State Sample unlabeled batch $(\overline{x}^i_k)$ from $\mathcal{D}_{OOD}$
        \State $l \gets l + \frac{1}{N} \mathcal{L}_{CE}(x^i_k, y^i_k; \theta_k) + \frac{\beta}{N} \mathcal{L}_{OE}(\overline{x}^i_k; \theta_k)$
    \EndFor
    \State Sample batch $(\hat x_k, \hat y_k)$ from $\mathcal{D}$
    \State $l \gets l + \lambda \mathcal{L}_{div}(\hat x_k, \hat y_k; \theta_1, \dots, \theta_N)$
    \For{$k \gets 1$ to $N$}
        \State $\theta_k \gets \theta_k - \epsilon \nabla_{\theta_k}l$
    \EndFor
\EndFor
\end{algorithmic}
\end{algorithm}
